# Supplementary material for: Unleashing the Potential of Differential Evolution through Individual-Level Strategy Diversity
Source: arXiv:2602.01147 source file (2026-02-01)
Supplement: Supplementary file 1 [file supp_diversity_distribution.tex]

\begin{figure*}[htpb]
\centering
\includegraphics[width=0.8\textwidth]{supp_figures/diversity_distribution.pdf}
\caption{\textbf{Statistical distribution of assigned strategies in iStratDE with a population size of $N=100,000$.} The bar charts and tables illustrate the counts for (a) Mutation strategies and (b) Crossover strategies. The results exhibit a near-perfect uniform distribution (indicated by the ``Ideal Uniform'' dashed lines), with entropy values virtually matching the theoretical maximums (1.99999 vs. 2.00000 for mutation, and 1.58495 vs. 1.58496 for crossover). This empirical evidence confirms that the large-scale random sampling mechanism effectively guarantees comprehensive structural diversity across the population.}
\label{Figure_strategy_diversity}
\end{figure*}
